# Supplementary material for: Partial Predicate Abstraction and Counter-Example Guided Refinement
Source: arXiv:1712.01734 source file (2017-12-05)
Supplement: Supplementary file 1 [file appendix.tex]

\begin{footnotesize}
Let $\bar{A}$ denote an ordered list of terms from set $A$. Let $cube^{\bar{A}}=\bigwedge_{k=1}^{|A|} 
a_k$, where $a_k \in A$ or $\neg a_k \in A$ and $k$ denotes the index of $a_k$ in $\bar{A}$.  Let $cube_{i}^{\bar{A}}$ denote the cube that
 evaluates to $i$ when regarded as a $|A|$ bit number when the terms' encoding are interpreted as 0
  for those that are negated and as 1 for the non-negated. For instance $cube^A_0$ denotes  $\bigwedge_{k=1}^{|A|} \neg a_k$, where $a_k \in A$. Also, let $|\varphi|=n$.
  
Lemma \ref{lemma:galoisState}.
%\vspace{-2cm}
%\end{footnotesize} 
\begin{proof} %\vspace{-2cm}
%\begin{footnotesize}
\begin{equation}
\begin{split}
   s \ \wedge \ cube^{\varphi}_i \ \to \ & \exists V_{\varphi}. s \ \wedge \ cube^{\varphi}_i  \ (\mbox{due to Existential Introduction})  \\
   s \ \wedge \ cube^{\varphi}_i \ \wedge \ cube^{\varphi}_i \to \ & (\exists V_{\varphi}. s \ \wedge \ cube^{\varphi}_i) \  \wedge \ cube^{\varphi}_i \\
      s \ \wedge \ cube^{\varphi}_i \ \to \ & (\exists V_{\varphi}. s \ \wedge \ cube^{\varphi}_i) \  \wedge \ cube^{\varphi}_i \\
   \bigvee^{2^n-1}_{i=0}   s \ \wedge \ cube^{\varphi}_i \ \to \ &  \bigvee^{2^n-1}_{i=0} (\exists V_{\varphi}. s \ \wedge \ cube^{\varphi}_i) \  \wedge \ cube^{\varphi}_i \\  
    s \ \wedge \  \bigvee^{2^n-1}_{i=0}  cube^{\varphi}_i \ \to \ &  \bigvee^{2^n-1}_{i=0} (\exists V_{\varphi}. s \ \wedge \ cube^{\varphi}_i) \  \wedge \ cube^{\varphi}_i \\  
   s \ \wedge \ true \ \to &  \ \bigvee^{2^n-1}_{i=0} (\exists V_{\varphi}. s \ \wedge \ cube^{\varphi}_i) \  \wedge \ cube^{\varphi}_i \\  
   s  \ \to & \  \bigvee^{2^n-1}_{i=0} (\exists V_{\varphi}. s \ \wedge \ cube^{\varphi}_i) \  \wedge \ cube^{\varphi}_i \\ 
           s \ \to  & \ (\bigvee^{2^n-1}_{i=0}  \exists V_{\varphi}. (s \ \wedge \ cube^{\varphi}_i) \ \wedge \ cube^{b}_i)) [\bar{\varphi}/\bar{b}]  \\   
                      s \ \to  & \ (\bigvee^{2^n-1}_{i=0}  \exists V_{\varphi}. (s \ \wedge \ cube^{\varphi}_i \ \wedge \ cube^{b}_i)) [\bar{\varphi}/\bar{b}]  \ 
                      (\mbox{due to } V_{\varphi} \cap V_b = \emptyset) \\   
                         s \ \to  & \ (\exists V_{\varphi}. (\bigvee^{2^n-1}_{i=0} s \ \wedge \  cube^{\varphi}_i \ \wedge \ cube^{b}_i)) [\bar{\varphi}/\bar{b}]  \\
    s \ \to  & \ (\exists V_{\varphi}. (s \ \wedge \ \bigvee^{2^n-1}_{i=0} cube^{\varphi}_i \ \wedge \ cube^{b}_i)) [\bar{\varphi}/\bar{b}]  \\
   s \ \to  & \ \gamma(\exists V_{\varphi}. (s \ \wedge \ \bigvee^{2^n-1}_{i=0} cube^{\varphi}_i \ \wedge \ cube^{b}_i)) \\   
   s \ \to  & \ \gamma(\exists V_{\varphi}. (s \ \wedge \ \bigwedge^{|\varphi|}_{j=1} \varphi_j \iff b_j)) \\    
   s \ \to & \ \gamma(\alpha(s))  \\
     \end{split}                  
\end{equation}
%\end{footnotesize}
\end{proof}
%\vspace{-2cm}

Lemma \ref{lemma:galoisTrans}.
%\vspace{-2cm}
\begin{proof} 
%\begin{footnotesize}
%\begin{itemize}
%\item  
{\bf Showing} $r^{\natural} \ \to \ \gamma^{\tau}(\alpha^{\tau}(r^{\natural}))$:
Also, let $\overline{\varphi''}$ and $\overline{b''}$ denote the ordered list of terms from the set $\varphi \cup \varphi'$ and the ordered list of terms from the set $b \cup b'$, respectively. Let $n=|\varphi|=|\varphi'|$ and $CS'=\bigwedge_{\varphi_i \in \varphi} ((\bigwedge_{v \in V(\varphi_i)} v'=v ) \implies \varphi'_i \iff \varphi_i)$.
\begin{equation*}
\begin{split}
   r^{\natural} \ \wedge \ CS' \ \wedge \ cube^{\overline{\varphi''}}_i \to \ & \exists V_{\varphi \cup \varphi'}. r^{\natural}  \ \wedge \ CS' \ \wedge \  cube^{\overline{\varphi''}}_i \ \\
   %(\mbox{due to Existential Introduction}) \\
   r^{\natural} \ \wedge \ CS' \ \wedge \ cube^{\overline{\varphi''}}_i \ \wedge \ cube^{\overline{\varphi''}}_i \to \ & (\exists V_{\varphi \cup \varphi'}. r^{\natural} \ \wedge \ CS' \ \wedge \  cube^{\overline{\varphi''}}_i) \  \wedge \ cube^{\overline{\varphi''}}_i \\
      r^{\natural} \ \wedge \ CS' \ \wedge \ cube^{\overline{\varphi''}}_i \ \to \ & (\exists V_{\varphi \cup \varphi'}. r^{\natural} \ \wedge \ CS' \ \wedge \  cube^{\overline{\varphi''}}_i) \  \wedge \ cube^{\overline{\varphi''}}_i \\
   \bigvee^{2^{2n}-1}_{i=0}   r^{\natural} \ \wedge \ CS' \ \wedge \ cube^{\overline{\varphi''}}_i \ \to \ &  \bigvee^{2^{2n}-1}_{i=0} (\exists V_{\varphi \cup \varphi'}. r^{\natural} \ \wedge \ CS' \ \wedge \ cube^{\overline{\varphi''}}_i) \  \wedge \ cube^{\overline{\varphi''}}_i \\  
%\end{split}
%\end{equation*}
%\begin{equation*}
%\begin{split}   
    r^{\natural} \ \wedge \ CS' \ \wedge \  \bigvee^{2^{2n}-1}_{i=0}  cube^{\overline{\varphi''}}_i \ \to \ &  \bigvee^{2^{2n}-1}_{i=0} (\exists V_{\varphi \cup \varphi'}. r^{\natural} \ \wedge \ CS' \ \wedge \ cube^{\overline{\varphi''}}_i) \  \wedge \ cube^{\overline{\varphi''}}_i \\  
   r^{\natural} \ \wedge \ true \ \to &  \ \bigvee^{2^{2n}-1}_{i=0} (\exists V_{\varphi \cup \varphi'}. r^{\natural} \ \wedge \ CS' \ \wedge \  cube^{\overline{\varphi''}}_i) \  \wedge \ cube^{\overline{\varphi''}}_i \\  
   r^{\natural}  \ \to & \  \bigvee^{2^{2n}-1}_{i=0} (\exists V_{\varphi \cup \varphi'}. r^{\natural} \ \wedge \ CS' \ \wedge \  cube^{\overline{\varphi''}}_i) \  \wedge \ cube^{\overline{\varphi''}}_i \\ 
           r^{\natural} \ \to  & \ (\bigvee^{2^{2n}-1}_{i=0}  \exists V_{\varphi \cup \varphi'}. (r^{\natural} \ \wedge \ CS \ \wedge \  cube^{\overline{\varphi''}}_i) \ \wedge \ cube^{\overline{b''}}_i)) [\overline{\varphi''}/\overline{b''}]  \\   
%\end{split}
%\end{equation*}
%\begin{equation*}
%\begin{split}              
                      r^{\natural} \ \to  & \ (\bigvee^{2^{2n}-1}_{i=0}  \exists V_{\varphi \cup \varphi'}. (r^{\natural} \ \wedge \ CS \ \wedge \  cube^{\overline{\varphi''}}_i \ \wedge \ cube^{\overline{b''}}_i)) [\bar{\overline{\varphi''}}/\overline{b''}]  \\
                      &  (\mbox{due to } V_{\varphi \cup \varphi'} \cap V_b = \emptyset) \\   
                         r^{\natural} \ \to  & \ (\exists V_{\varphi \cup \varphi'}. (\bigvee^{2^{2n}-1}_{i=0} r^{\natural} \ \wedge \ CS \ \wedge \   cube^{\overline{\varphi''}}_i \ \wedge \ cube^{\overline{b''}}_i)) [\overline{\varphi''}/\overline{b''}]  \\
    r^{\natural} \ \to  & \ (\exists V_{\varphi \cup \varphi'}. (r^{\natural} \ \wedge \ CS \ \wedge \  \bigvee^{2^{2n}-1}_{i=0} cube^{\overline{\varphi''}}_i \ \wedge \ cube^{\overline{b''}}_i)) [\overline{\varphi''}/\overline{b''}]  \\
%\end{split}
%\end{equation*}
%\begin{equation}
%\begin{split}        
   r^{\natural} \ \to  & \ \gamma^{\tau}(\exists V_{\varphi \cup \varphi'}. (r^{\natural} \ \wedge \ CS \ \wedge \ \bigvee^{2^{2n}-1}_{i=0} cube^{\overline{\varphi''}}_i \ \wedge \ cube^{\overline{b''}}_i)) \\   
   r^{\natural} \ \to  & \ \gamma^{\tau}(\exists V_{\varphi \cup \varphi'}. (r^{\natural} \ \wedge \ CS \ \wedge \  \bigwedge^{|\varphi|}_{j=1} \varphi_j \iff b_j  \ \wedge \ \bigwedge^{|\varphi'|}_{j=1} \varphi'_j \iff b'_j )) \\    
   r^{\natural} \ \to & \ \gamma^{\tau}(\alpha^{\tau}(r^{\natural}))  \\
\end{split}
%\begin{proof}
%The proof is similar to the steps taken in the sequence of Proof of Lemma \ref{lemma:galoisState}, where $cube^{\varphi}_i$ and $cube^{b}_i$ are replaced with $cube^{\varphi+\varphi'}_i$ and $cube^{b+b'}_i$, respectively.
%\end{proof}
\end{equation*}
%\item 
{\bf Showing} $r^{\sharp}=\alpha(\gamma(r^{\sharp}))$:
\begin{equation}
\begin{split}
 \equiv \ & \alpha(\gamma(r^{\sharp})) \\
\equiv \ & \exists V(\varphi). \exists V(\varphi'). (r^{\sharp} [\bar{\varphi},\bar{\varphi}'/\bar{b},\bar{b}'] \ \wedge \ CS \ \wedge \ \bigwedge^{|\varphi|}_{i=1} \varphi_i \iff b_i \wedge \ \bigwedge^{|\varphi|}_{i=1} \varphi_i' \iff b_i'  )\\ 
\equiv \ & \exists V(\varphi). \exists V(\varphi'). (r^{\sharp} [\bar{\varphi},\bar{\varphi}'/\bar{b},\bar{b}'] \ \wedge \ \bigwedge^{|\varphi|}_{i=1} \varphi_i \iff b_i \wedge \ \bigwedge^{|\varphi|}_{i=1} \varphi_i' \iff b_i'  ) \\
%& (CS \mbox{ will preserve any identity relation } (b'_i=b_i)  \mbox{ in } r^{\sharp} \mbox{ and will trivially evaluate} \\
%& \mbox{to true in the case of } b'_i\not=b_i )\\
\equiv \ & r^{\sharp} \\
\end{split}
\end{equation}
%\end{itemize}
%\end{footnotesize}
\end{proof}
\end{footnotesize}
%\vspace{-1cm}
